# Supplementary material for: Hierarchical Memory Matching Network for Video Object Segmentation
Source: arXiv:2109.11404 source file (2021-09-23)
Supplement: Supplementary file 2 [file supp.pdf]

# Supplementary Material: Hierarchical Memory Matching Network for Video Object Segmentation

Hongje Seong<sup>1</sup>   Seoung Wug Oh<sup>2</sup>   Joon-Young Lee<sup>2</sup>  
 Seongwon Lee<sup>1</sup>   Suhyeon Lee<sup>1</sup>   Euntai Kim<sup>1,\*</sup>  
<sup>1</sup>Yonsei University   <sup>2</sup>Adobe Research

## 1. Network Structure Details

**Top- $k$  guided memory matching module at res2 stage.** Fig. 1 shows a detailed implementation of the top- $k$  guided memory matching module at the res2 stage. Compare to the top- $k$  guided memory matching module at the res3 stage, we reduce the number of  $k$  to  $k/4$ . We also take the reduced channel dimensions of **key** and **value**, except for the query **value**.

**Detailed implementation of decoder.** We follow the decoder architecture of STM [24], and a detailed implementation is provided in Fig. 2. Note that, in the refinement modules of STM [24], the skip-connected features ( $Z_3, Z_2$ ) are encoded via convolutional layers before fed to residual block. We replace the convolutional layers with **value** embedding layers in top- $k$  guided memory matching modules.

## 2. More Quantitative Results

Tables 1, 2, and 3 provide full comparisons on DAVIS 2016 val, 2017 val, and 2017 test-dev sets, respectively. As shown in the tables, recent offline-learning methods such as KMN [27], CFBI [33], LWL [2], and STM [24] surpassed online-learning methods such as PReMVOS [20], RaNet [30], e-OSVOS [22], and DyeNet [14] by additionally using YouTube-VOS [31] training data. However, we surpass all online-learning methods, which need additional run-time for fine-tuning during inference, even if we do not use additional YouTube-VOS training data. Therefore, the superiority of our HMMN has not relied on additional YouTube-VOS training data.

## 3. More Qualitative Results

We show more qualitative results on DAVIS [25] in Fig. 3 and results on YouTube-VOS [31] in Figs. 4 and 5. In the figures, we additionally show the results of STM<sup>1</sup> [24],

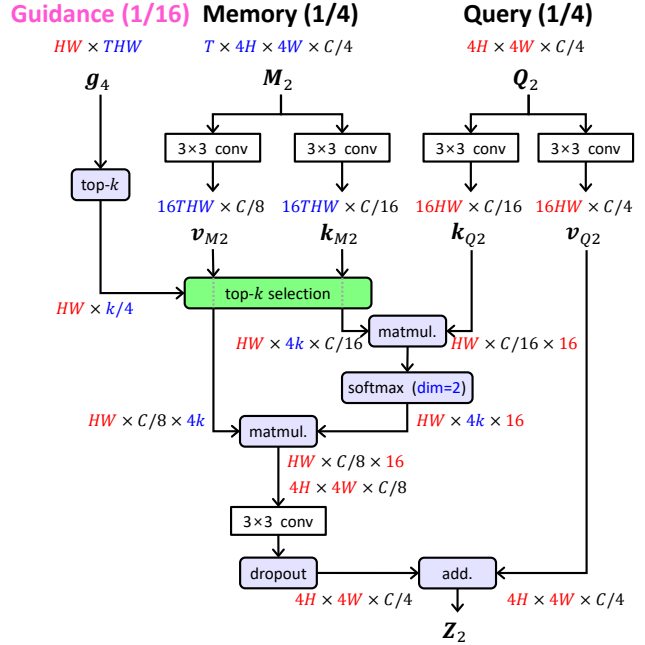

Figure 1. A detailed implementation of the top- $k$  guided memory matching module at the res2 stage. Memory and query dimensions are indicated using blue and red.

KMN<sup>2</sup> [27], and CFBI<sup>3</sup> [33]. Since some frames are omitted in the figures, we further provide a comparison video: <https://youtu.be/zSofRzPImQY>.

## References

- [1] Linchao Bao, Baoyuan Wu, and Wei Liu. Cnn in mrf: Video object segmentation via inference in a cnn-based higher-order spatio-temporal mrf. In *CVPR*, pages 5977–5986, 2018. 2, 6
- [2] Goutam Bhat, Felix Järemo Lawin, Martin Danelljan, Andreas Robinson, Michael Felsberg, Luc Van Gool, and Radu

\*Corresponding author.

<sup>1</sup>results are taken from <https://github.com/seoungwugoh/STM>.

<sup>2</sup>results are extracted from our reproduced model.

<sup>3</sup>results are taken from <https://github.com/z-x-yang/CFBI>.

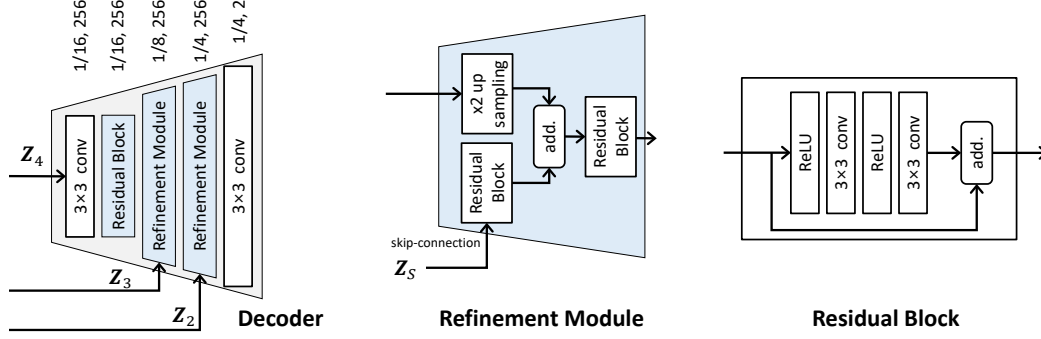

Figure 2. A detailed implementation of decoder. We notated the output scale and channel dimension next to each block in the decoder.

| Method                  | OL | $\mathcal{J}\&\mathcal{F}$ | $\mathcal{J}$ | $\mathcal{F}$ | Time  |
|-------------------------|----|----------------------------|---------------|---------------|-------|
| OSVOS [3]               | ✓  | 80.2                       | 79.8          | 80.6          | 9s    |
| MaskRNN [9]             | ✓  | 80.8                       | 80.7          | 80.9          | -     |
| VidMatch [10]           | -  | -                          | 81.0          | -             | 0.32s |
| FAVOS [5]               | -  | 81.0                       | 82.4          | 79.5          | 1.8s  |
| LSE [6]                 | ✓  | 81.6                       | 82.9          | 80.3          | -     |
| FEELVOS [28]            | -  | 81.7                       | 80.3          | 83.1          | 0.45s |
| FEELVOS (+YV) [28]      | -  | 81.7                       | 81.1          | 82.2          | 0.45s |
| FRTM [26]               | ✓  | 81.7                       | -             | -             | 0.05s |
| RGMP [23]               | -  | 81.8                       | 81.5          | 82.0          | 0.13s |
| A-GAME (+YV) [12]       | -  | -                          | 82.0          | -             | 0.07s |
| SAT [4]                 | -  | 83.1                       | 82.6          | 83.6          | 0.03s |
| FRTM (+YV) [26]         | ✓  | 83.5                       | -             | -             | 0.05s |
| DTN [35]                | -  | 83.6                       | 83.7          | 83.5          | 0.07s |
| CINN [1]                | ✓  | 84.2                       | 83.4          | 85.0          | >30s  |
| DyeNet [14]             | -  | -                          | 84.7          | -             | 0.42s |
| RaNet [30]              | -  | 85.5                       | 85.5          | 85.4          | 0.03s |
| OnAVOS [29]             | ✓  | 85.5                       | 86.1          | 84.9          | 13s   |
| STG-Net [18]            | -  | 85.7                       | 85.4          | 86.0          | 0.16s |
| OSVOS <sup>S</sup> [21] | ✓  | 86.0                       | 85.6          | 86.4          | 4.5s  |
| DIPNet [8]              | ✓  | 86.1                       | 85.8          | 86.4          | 1.09s |
| CFBI [33]               | -  | 86.1                       | 85.3          | 86.9          | 0.18s |
| STM [24]                | -  | 86.5                       | 84.8          | 88.1          | 0.16s |
| PreMVOS [20]            | ✓  | 86.8                       | 84.9          | 88.6          | 32.8s |
| e-OSVOS [22]            | ✓  | 86.8                       | 86.6          | 87.0          | 3.4s  |
| DyeNet [14]             | ✓  | -                          | 86.2          | -             | 2.32s |
| RaNet [30]              | ✓  | 87.1                       | 86.6          | 87.6          | 4s    |
| KMN [27]                | -  | 87.6                       | 87.1          | 88.1          | 0.12s |
| STM (+YV) [24]          | -  | 89.3                       | 88.7          | 89.9          | 0.16s |
| CFBI (+YV) [33]         | -  | 89.4                       | 88.3          | 90.5          | 0.18s |
| KMN (+YV) [27]          | -  | 90.5                       | 89.5          | 91.5          | 0.12s |
| HMMN                    | -  | 89.4                       | 88.2          | 90.6          | 0.10s |
| HMMN (+YV)              | -  | <b>90.8</b>                | <b>89.6</b>   | <b>92.0</b>   | 0.10s |

Table 1. Full comparison on DAVIS 2016 validation set. (+YV) indicates YouTube-VOS is additionally used for training, and OL denotes the use of online-learning strategies during test-time. Time measurements reported in this table are directly from the corresponding papers.

| Method                  | OL | $\mathcal{J}\&\mathcal{F}$ | $\mathcal{J}$ | $\mathcal{F}$ |
|-------------------------|----|----------------------------|---------------|---------------|
| OSVOS [3]               | ✓  | 60.3                       | 56.6          | 63.9          |
| VidMatch [10]           | -  | 62.4                       | 56.5          | 68.2          |
| MaskRNN [9]             | ✓  | -                          | 60.5          | -             |
| RaNet [30]              | -  | 65.7                       | 63.2          | 68.2          |
| AGSS-VOS [17]           | -  | 66.6                       | 63.4          | 69.8          |
| RGMP [23]               | -  | 66.7                       | 64.8          | 68.6          |
| DTN [35]                | -  | 67.4                       | 64.2          | 70.6          |
| AGSS-VOS (+YV) [17]     | -  | 67.4                       | 64.9          | 69.9          |
| OnAVOS [29]             | ✓  | 67.9                       | 64.5          | 71.2          |
| OSVOS <sup>S</sup> [21] | ✓  | 68.0                       | 64.7          | 71.3          |
| DIPNet [8]              | ✓  | 68.5                       | 65.3          | 71.6          |
| FRTM [26]               | ✓  | 68.8                       | -             | -             |
| FEELVOS [28]            | -  | 69.1                       | 65.9          | 72.3          |
| DyeNet [14]             | -  | 69.1                       | 67.3          | 71.0          |
| A-GAME (+YV) [12]       | -  | 70.0                       | 67.2          | 72.7          |
| CINN [1]                | ✓  | 70.7                       | 67.2          | 74.2          |
| DMM-Net [34]            | -  | 70.7                       | 68.1          | 73.3          |
| GC [15]                 | -  | 71.4                       | 69.3          | 73.5          |
| STM [24]                | -  | 71.6                       | 69.2          | 74.0          |
| FEELVOS (+YV) [28]      | -  | 72.0                       | 69.1          | 74.0          |
| SAT [4]                 | -  | 72.3                       | 68.6          | 76.0          |
| TVOS [36]               | -  | 72.3                       | 69.9          | 74.7          |
| LWL [2]                 | -  | 74.3                       | 72.2          | 76.3          |
| AFB+URR [16]            | -  | 74.6                       | 73.0          | 76.1          |
| STG-Net [18]            | -  | 74.7                       | 71.5          | 77.9          |
| CFBI [33]               | -  | 74.9                       | 72.1          | 77.7          |
| DTTM-TAN [11]           | -  | 75.9                       | 72.3          | 79.4          |
| KMN [27]                | -  | 76.0                       | 74.2          | 77.8          |
| FRTM (+YV) [26]         | ✓  | 76.7                       | -             | -             |
| e-OSVOS [22]            | ✓  | 77.2                       | 74.4          | 80.0          |
| PreMVOS [20]            | ✓  | 77.8                       | 73.9          | 81.7          |
| LWL (+YV) [2]           | -  | 81.6                       | 79.1          | 84.1          |
| STM (+YV) [24]          | -  | 81.8                       | 79.2          | 84.3          |
| CFBI (+YV) [33]         | -  | 81.9                       | 79.1          | 84.6          |
| EGMN (+YV) [19]         | -  | 82.8                       | 80.2          | 85.2          |
| KMN (+YV) [27]          | -  | 82.8                       | 80.0          | 85.6          |
| HMMN                    | -  | 80.4                       | 77.7          | 83.1          |
| HMMN (+YV)              | -  | <b>84.7</b>                | <b>81.9</b>   | <b>87.5</b>   |

Table 2. Full comparison on DAVIS 2017 validation set.

Timofte. Learning what to learn for video object segmentation. In *ECCV*, 2020. 1, 2

[3] Sergi Caelles, Kevis-Kokitsi Maninis, Jordi Pont-Tuset, Laura Leal-Taixé, Daniel Cremers, and Luc Van Gool. One-shot video object segmentation. In *CVPR*, pages 221–230,

2017. 2, 6

[4] Xi Chen, Zuoxin Li, Ye Yuan, Gang Yu, Jianxin Shen, and Donglian Qi. State-aware tracker for real-time video object segmentation. In *CVPR*, pages 9384–9393, 2020. 2

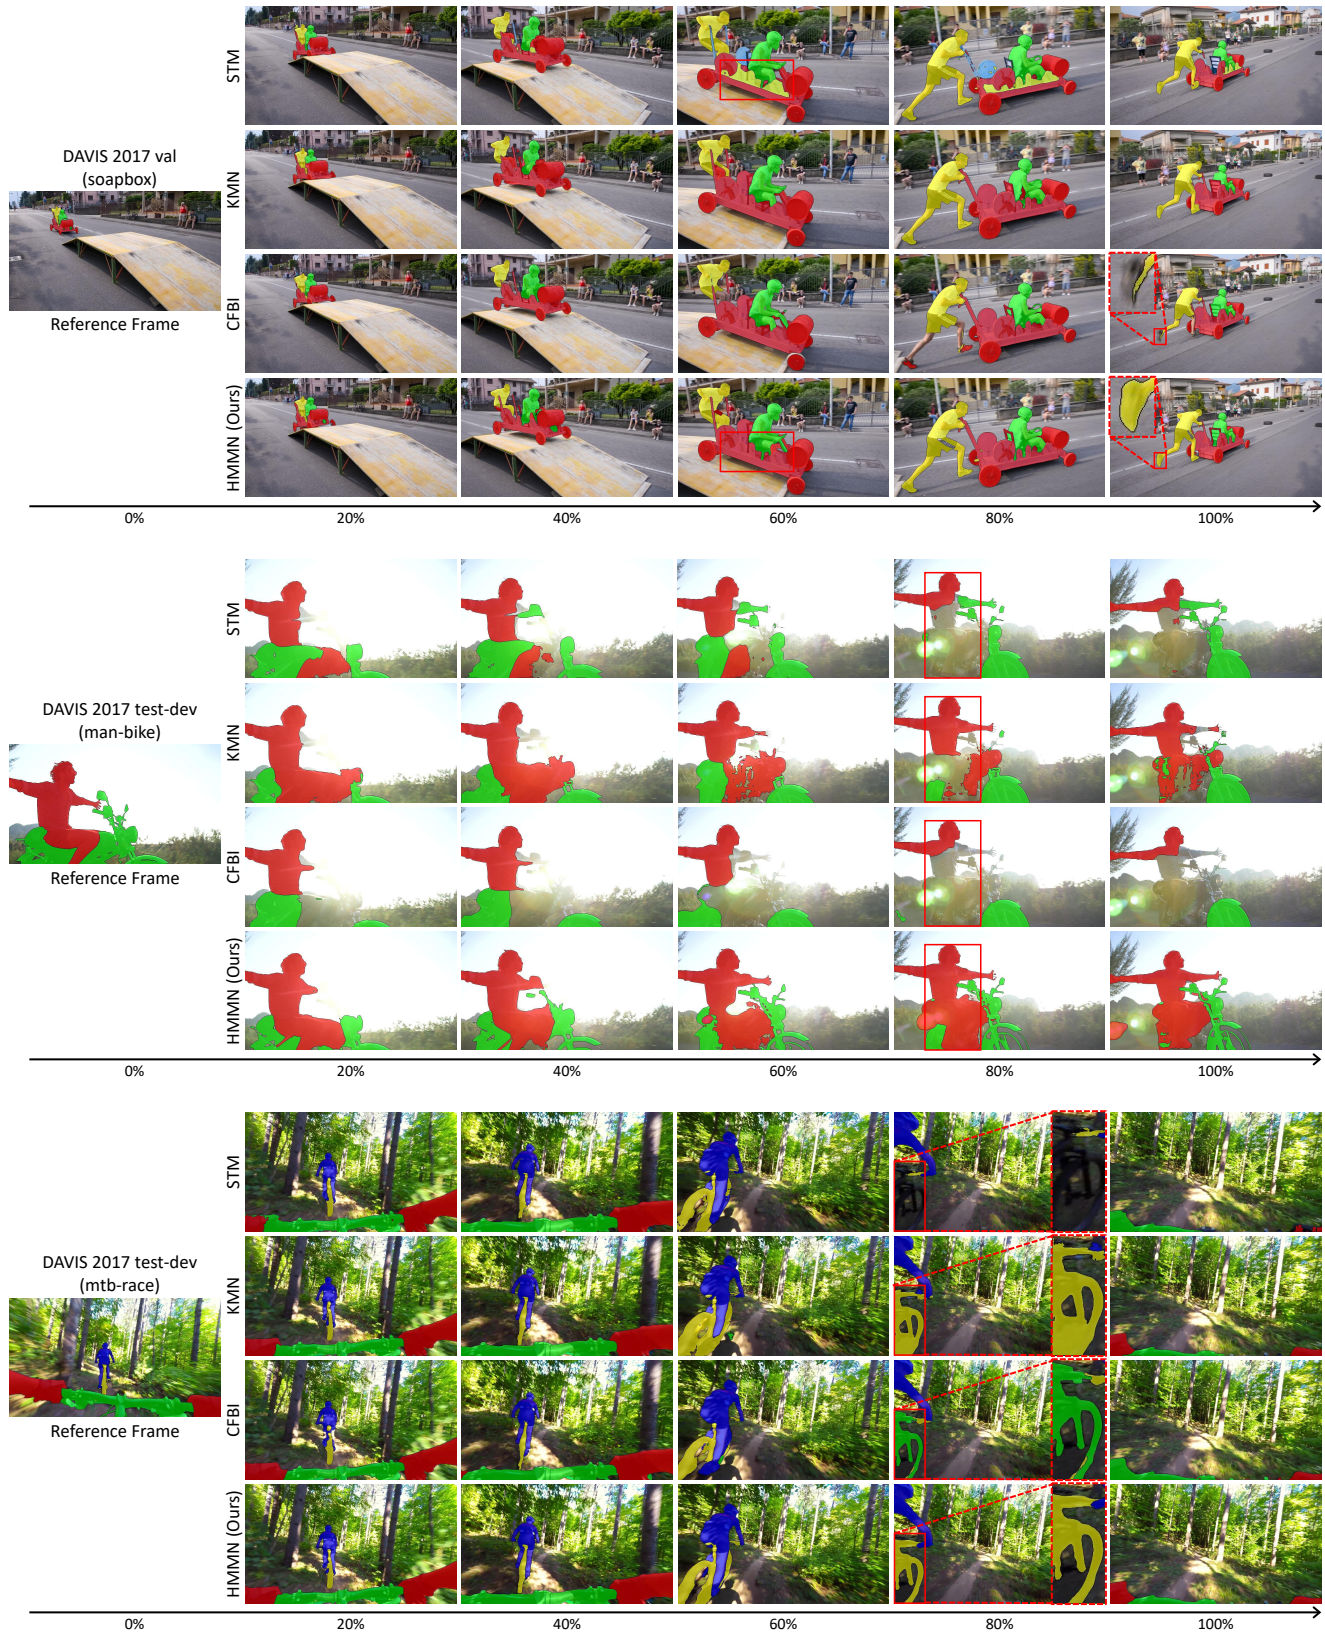

Figure 3. More qualitative results on DAVIS 2017 validation and test-dev sets. We marked significant improvements from STM [24], KMN [27], and CFBI [33] using red boxes.



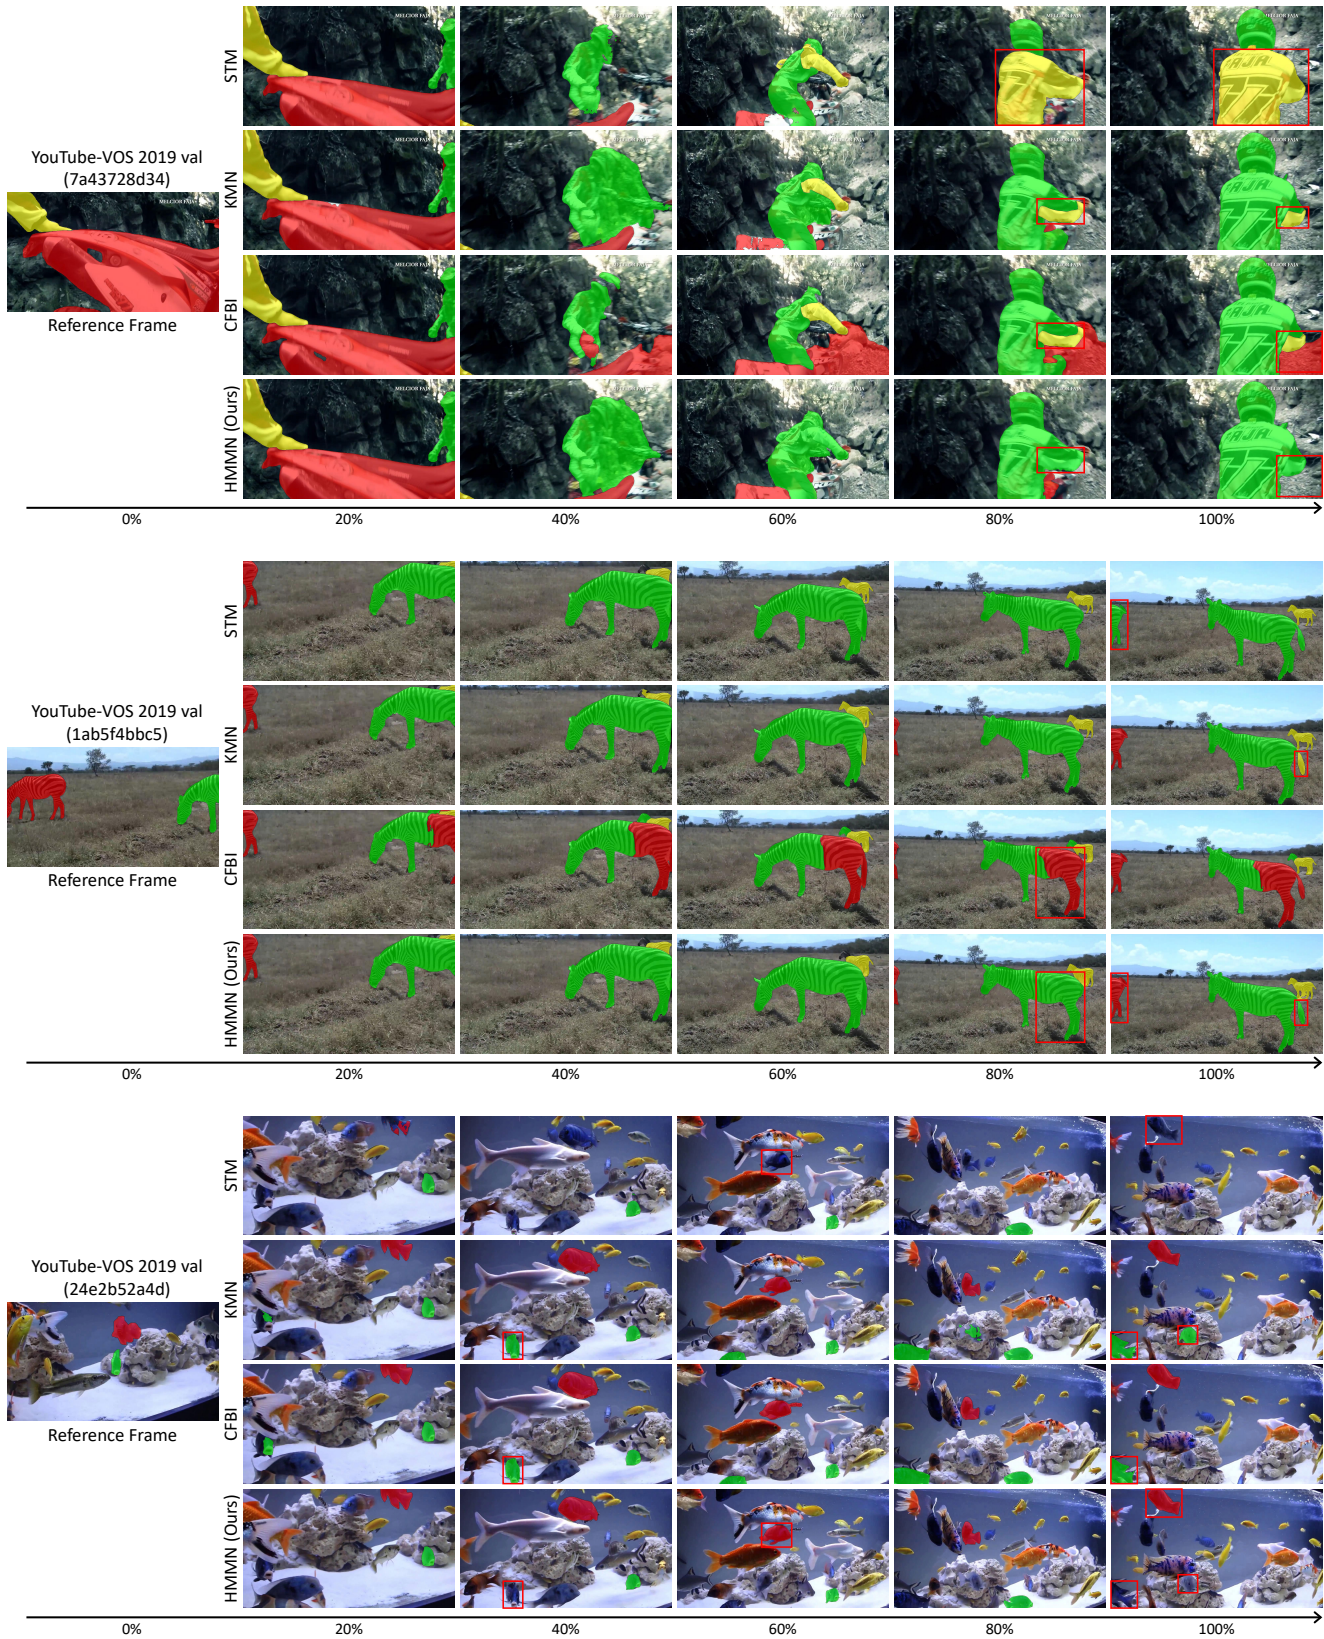

Figure 4. More qualitative results on YouTube-VOS 2019 validation set.



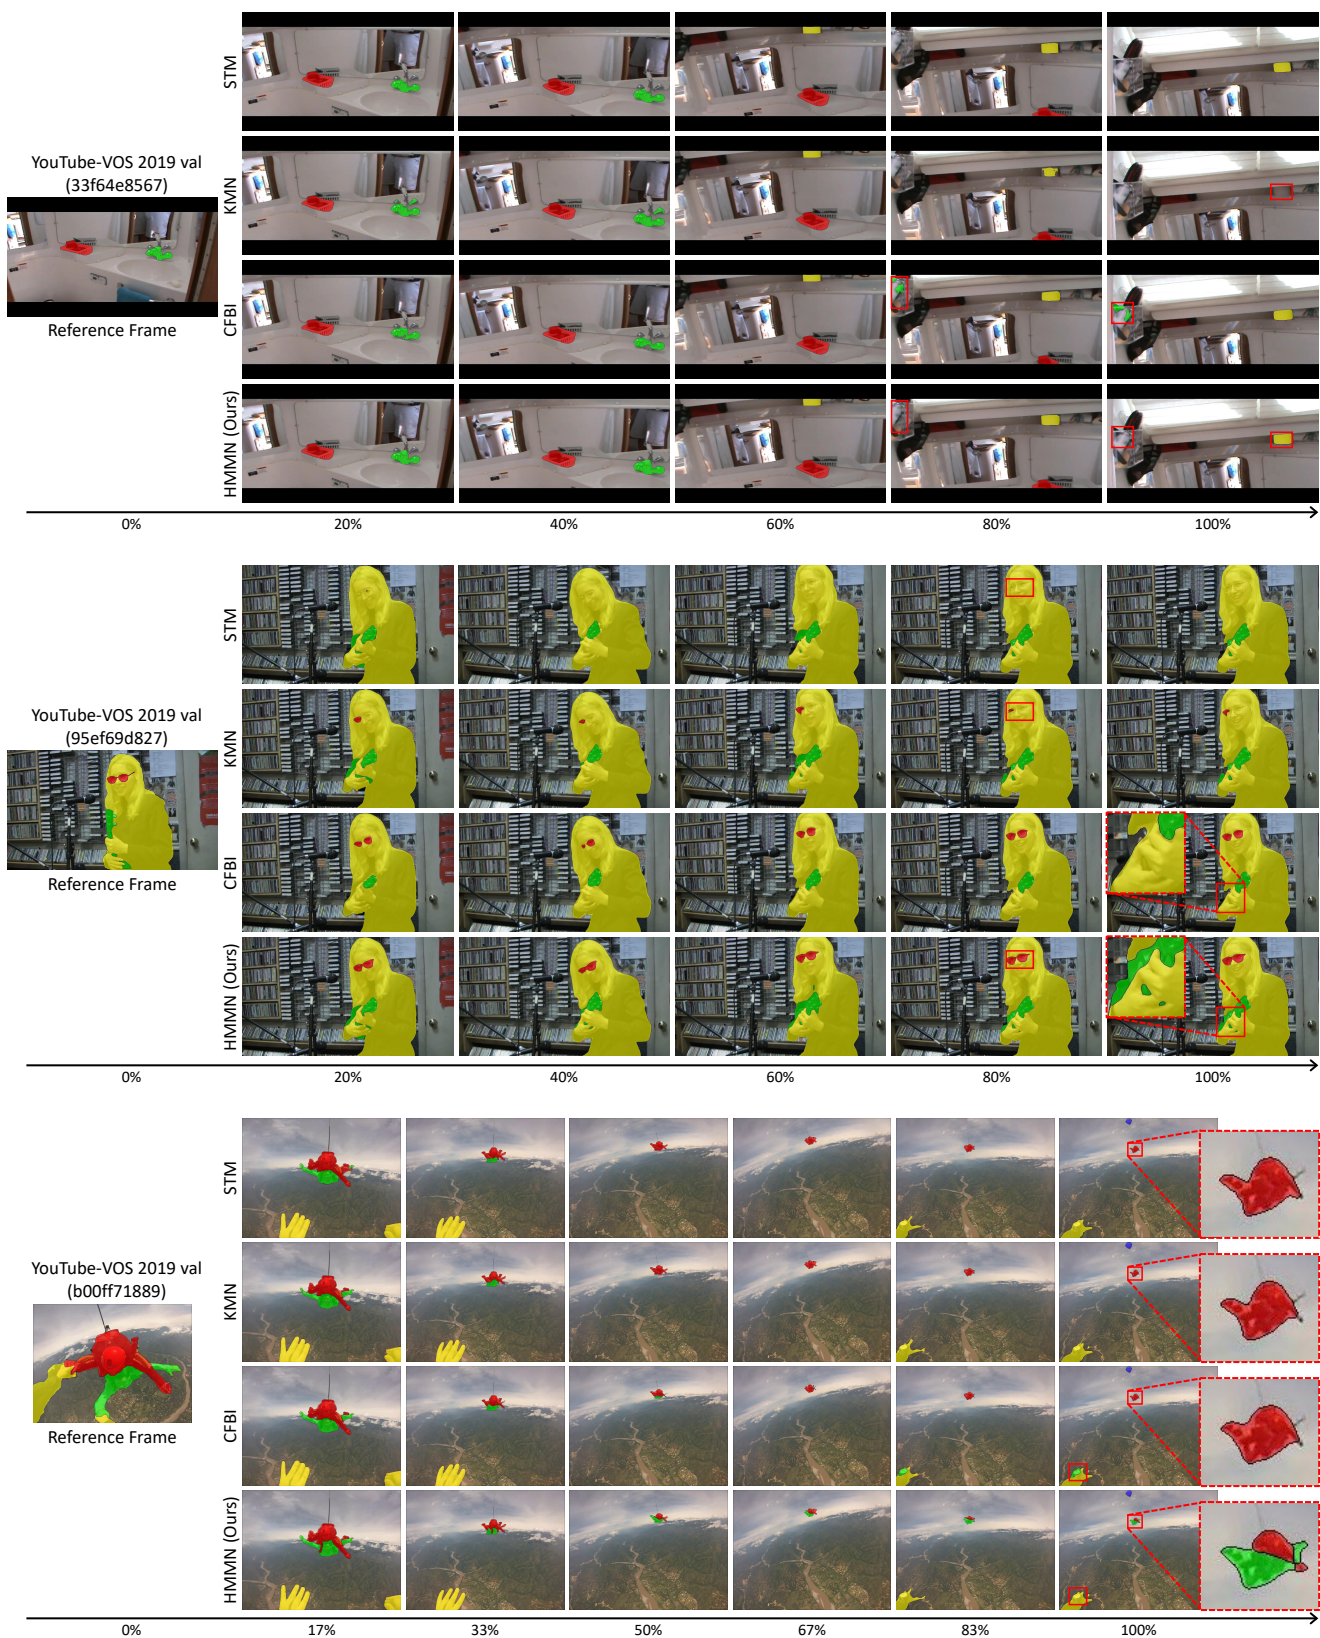

Figure 5. More qualitative results on YouTube-VOS 2019 validation set.

| Method                  | OL | $\mathcal{J}\&\mathcal{F}$ | $\mathcal{J}$ | $\mathcal{F}$ |
|-------------------------|----|----------------------------|---------------|---------------|
| OSMN [32]               |    | 39.3                       | 33.7          | 44.9          |
| FAVOS [5]               |    | 43.6                       | 42.9          | 44.2          |
| OSVOS [3]               | ✓  | 50.9                       | 47.0          | 54.8          |
| CapsuleVOS [7]          |    | 51.3                       | 47.4          | 55.2          |
| OnAVOS [29]             | ✓  | 52.8                       | 49.9          | 55.7          |
| RGMP [23]               |    | 52.9                       | 51.3          | 54.4          |
| RaNet [30]              |    | 53.4                       | 55.3          | 57.2          |
| OSVOS <sup>S</sup> [21] | ✓  | 57.5                       | 52.9          | 62.1          |
| FEELVOS (+YV) [28]      |    | 57.8                       | 55.1          | 60.4          |
| TVOS [36]               |    | 63.1                       | 58.8          | 67.4          |
| STG-Net [18]            |    | 63.1                       | 59.7          | 66.5          |
| e-OSVOS [22]            | ✓  | 64.8                       | 60.9          | 68.6          |
| DTTM-TAN [11]           |    | 65.4                       | 61.3          | 70.3          |
| Lucid [13]              | ✓  | 66.7                       | 63.4          | 69.9          |
| CINN [1]                | ✓  | 67.5                       | 64.5          | 70.5          |
| DyeNet [14]             | ✓  | 68.2                       | 65.8          | 70.5          |
| PRemVOS [20]            | ✓  | 71.6                       | 67.5          | 75.7          |
| STM (+YV) [24]          |    | 72.2                       | 69.3          | 75.2          |
| CFBI (+YV) [33]         |    | 74.8                       | 71.1          | 78.5          |
| KMN (+YV) [27]          |    | 77.2                       | 74.1          | 80.3          |
| <b>HMMN (+YV)</b>       |    | <b>78.6</b>                | <b>74.7</b>   | <b>82.5</b>   |

Table 3. Full comparison on DAVIS 2017 test-dev set.

- [5] Jingchun Cheng, Yi-Hsuan Tsai, Wei-Chih Hung, Shengjin Wang, and Ming-Hsuan Yang. Fast and accurate online video object segmentation via tracking parts. In *CVPR*, pages 7415–7424, 2018. 2, 6
- [6] Hai Ci, Chunyu Wang, and Yizhou Wang. Video object segmentation by learning location-sensitive embeddings. In *ECCV*, pages 501–516, 2018. 2
- [7] Kevin Duarte, Yogesh S. Rawat, and Mubarak Shah. Capsulevos: Semi-supervised video object segmentation using capsule routing. In *ICCV*, October 2019. 6
- [8] Ping Hu, Jun Liu, Gang Wang, Vitaly Ablavsky, Kate Saenko, and Stan Sclaroff. Dipnet: Dynamic identity propagation network for video object segmentation. In *WACV*, pages 1904–1913, 2020. 2
- [9] Yuan-Ting Hu, Jia-Bin Huang, and Alexander Schwing. Maskrnn: Instance level video object segmentation. In *NIPS*, pages 325–334, 2017. 2
- [10] Yuan-Ting Hu, Jia-Bin Huang, and Alexander G Schwing. Videomatch: Matching based video object segmentation. In *ECCV*, pages 54–70, 2018. 2
- [11] Xuhua Huang, Jiarui Xu, Yu-Wing Tai, and Chi-Keung Tang. Fast video object segmentation with temporal aggregation network and dynamic template matching. In *CVPR*, pages 8879–8889, 2020. 2, 6
- [12] Joakim Johnander, Martin Danelljan, Emil Brissman, Fahad Shahbaz Khan, and Michael Felsberg. A generative appearance model for end-to-end video object segmentation. In *CVPR*, pages 8953–8962, 2019. 2
- [13] Anna Khoreva, Rodrigo Benenson, Eddy Ilg, Thomas Brox, and Bernt Schiele. Lucid data dreaming for video object segmentation. *International Journal of Computer Vision*, 127(9):1175–1197, 2019. 6
- [14] Xiaoxiao Li and Chen Change Loy. Video object segmentation with joint re-identification and attention-aware mask propagation. In *ECCV*, pages 90–105, 2018. 1, 2, 6
- [15] Yu Li, Zhuoran Shen, and Ying Shan. Fast video object segmentation using the global context module. In *ECCV*, 2020. 2
- [16] Yongqing Liang, Xin Li, Navid Jafari, and Qin Chen. Video object segmentation with adaptive feature bank and uncertain-region refinement. In *NIPS*, 2020. 2
- [17] Huaijia Lin, Xiaojuan Qi, and Jiaya Jia. Agss-vos: Attention guided single-shot video object segmentation. In *ICCV*, October 2019. 2
- [18] Daizong Liu, Shuangjie Xu, Xiao-Yang Liu, Zichuan Xu, Wei Wei, and Pan Zhou. Spatiotemporal graph neural network based mask reconstruction for video object segmentation. In *AAAI*, 2021. 2, 6
- [19] Xinkai Lu, Wenguan Wang, Martin Danelljan, Tianfei Zhou, Jianbing Shen, and Luc Van Gool. Video object segmentation with episodic graph memory networks. In *ECCV*, 2020. 2
- [20] Jonathon Luiten, Paul Voigtlaender, and Bastian Leibe. Pre-mvos: Proposal-generation, refinement and merging for video object segmentation. In *ACCV*, pages 565–580. Springer, 2018. 1, 2, 6
- [21] K-K Maninis, Sergi Caelles, Yuhua Chen, Jordi Pont-Tuset, Laura Leal-Taixé, Daniel Cremers, and Luc Van Gool. Video object segmentation without temporal information. *IEEE Transactions on Pattern Analysis and Machine Intelligence*, 41(6):1515–1530, 2019. 2, 6
- [22] Tim Meinhardt and Laura Leal-Taixé. Make one-shot video object segmentation efficient again. In *NIPS*, 2020. 1, 2, 6
- [23] Seoung Wug Oh, Joon-Young Lee, Kalyan Sunkavalli, and Seon Joo Kim. Fast video object segmentation by reference-guided mask propagation. In *CVPR*, pages 7376–7385, 2018. 2, 6
- [24] Seoung Wug Oh, Joon-Young Lee, Ning Xu, and Seon Joo Kim. Video object segmentation using space-time memory networks. In *ICCV*, October 2019. 1, 2, 3, 6
- [25] Jordi Pont-Tuset, Federico Perazzi, Sergi Caelles, Pablo Arbeláez, Alex Sorkine-Hornung, and Luc Van Gool. The 2017 davis challenge on video object segmentation. *arXiv preprint arXiv:1704.00675*, 2017. 1
- [26] Andreas Robinson, Felix Jaremo Lawin, Martin Danelljan, Fahad Shahbaz Khan, and Michael Felsberg. Learning fast and robust target models for video object segmentation. In *CVPR*, pages 7406–7415, 2020. 2
- [27] Hongje Seong, Junhyuk Hyun, and Euntai Kim. Kernelized memory network for video object segmentation. In *ECCV*, 2020. 1, 2, 3, 6
- [28] Paul Voigtlaender, Yuning Chai, Florian Schroff, Hartwig Adam, Bastian Leibe, and Liang-Chieh Chen. Feelvos: Fast end-to-end embedding learning for video object segmentation. In *CVPR*, pages 9481–9490, 2019. 2, 6
- [29] Paul Voigtlaender and Bastian Leibe. Online adaptation of convolutional neural networks for video object segmentation. In *BMVC*, 2017. 2, 6



- [30] Ziqin Wang, Jun Xu, Li Liu, Fan Zhu, and Ling Shao. Ranet: Ranking attention network for fast video object segmentation. In *ICCV*, October 2019. 1, 2, 6
- [31] Ning Xu, Linjie Yang, Yuchen Fan, Jianchao Yang, Dingcheng Yue, Yuchen Liang, Brian Price, Scott Cohen, and Thomas Huang. Youtube-vos: Sequence-to-sequence video object segmentation. In *ECCV*, pages 585–601, 2018. 1
- [32] Linjie Yang, Yanran Wang, Xuehan Xiong, Jianchao Yang, and Aggelos K Katsaggelos. Efficient video object segmentation via network modulation. In *CVPR*, pages 6499–6507, 2018. 6
- [33] Zongxin Yang, Yunchao Wei, and Yi Yang. Collaborative video object segmentation by foreground-background integration. In *ECCV*, 2020. 1, 2, 3, 6
- [34] Xiaohui Zeng, Renjie Liao, Li Gu, Yuwen Xiong, Sanja Fidler, and Raquel Urtasun. Dmm-net: Differentiable mask-matching network for video object segmentation. In *ICCV*, October 2019. 2
- [35] Lu Zhang, Zhe Lin, Jianming Zhang, Huchuan Lu, and You He. Fast video object segmentation via dynamic targeting network. In *ICCV*, October 2019. 2
- [36] Yizhuo Zhang, Zhirong Wu, Houwen Peng, and Stephen Lin. A transductive approach for video object segmentation. In *CVPR*, pages 6949–6958, 2020. 2, 6
